# Supplementary material for: Parameterize Structure with Differentiable Template for 3D Shape Generation
Source: arXiv:2410.10399 source file (2024-10-15)

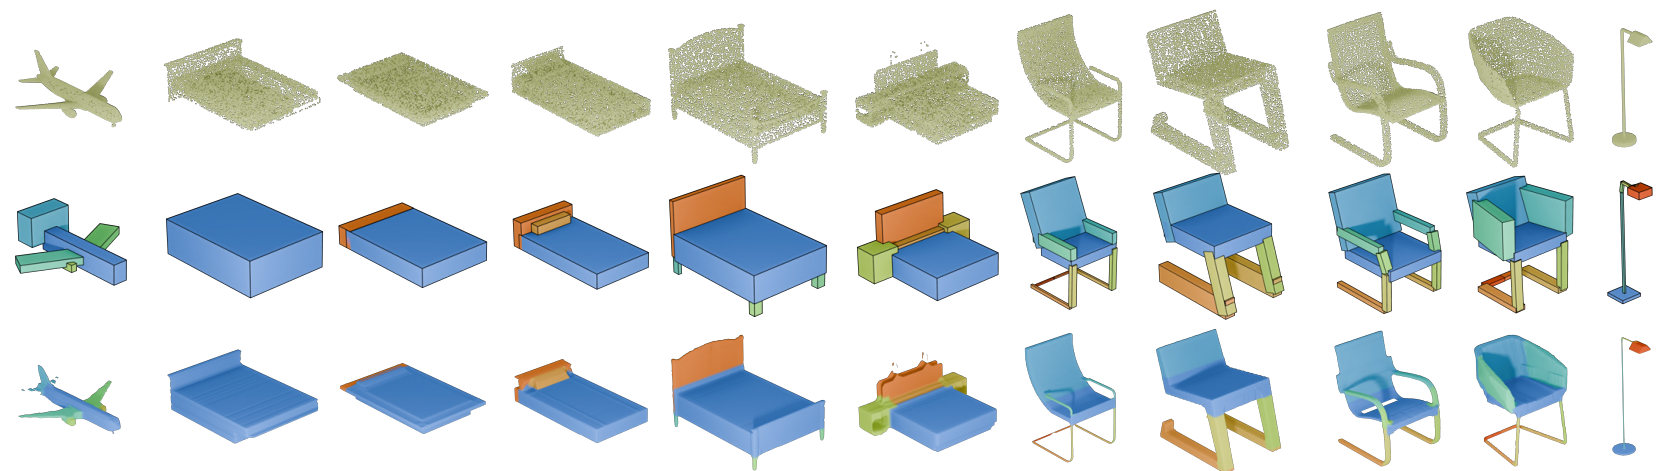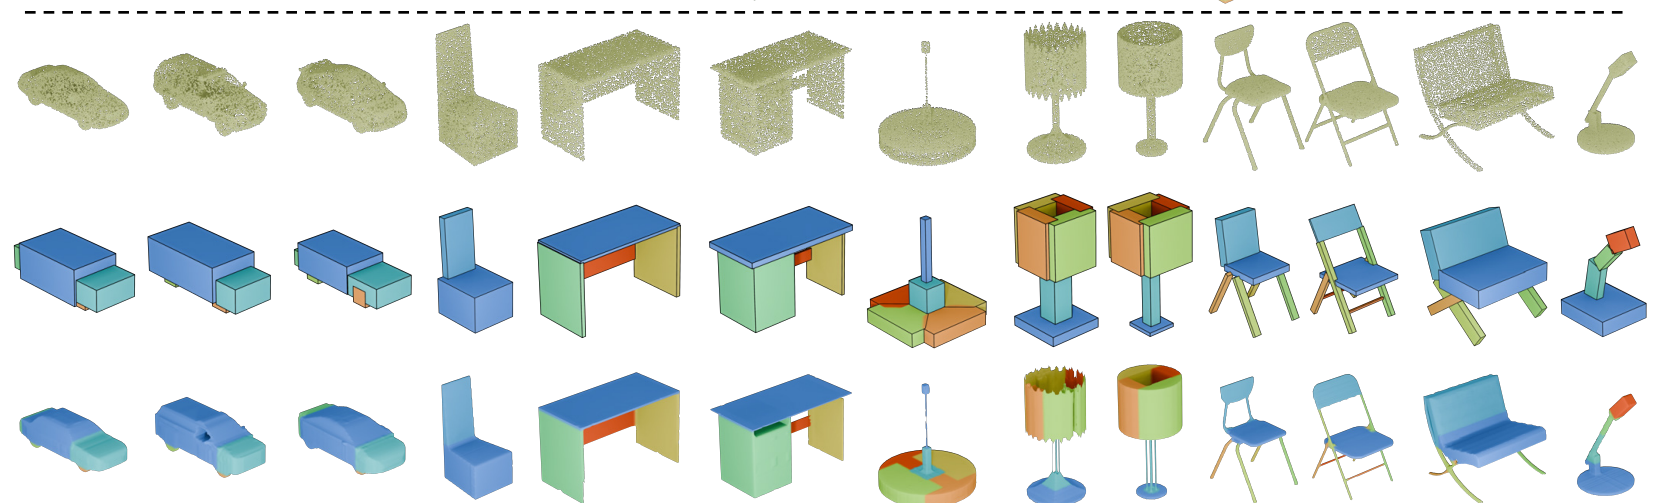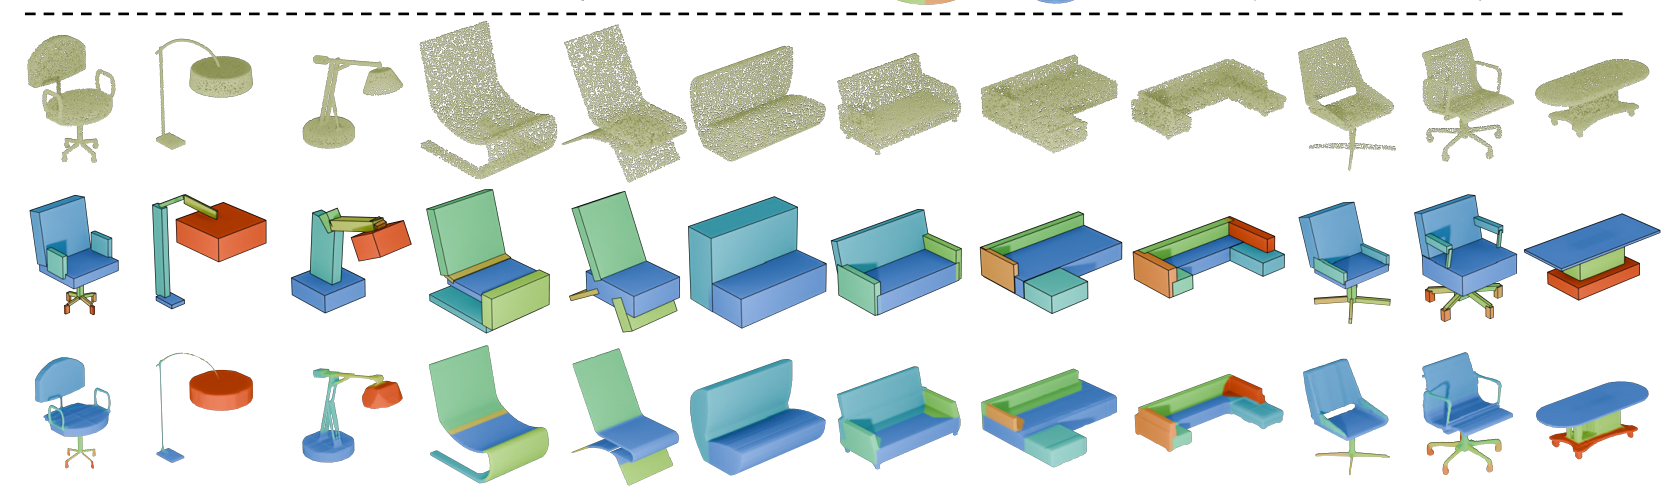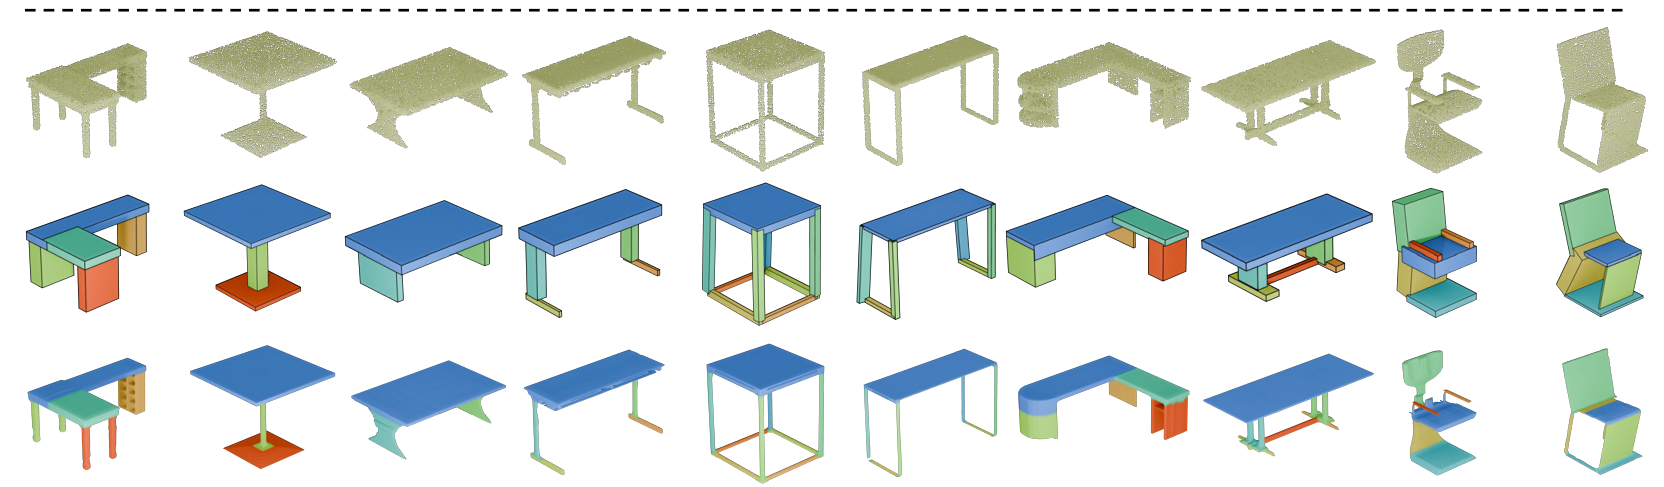

Supplement: Supplementary file 2 [file supp_recon.pdf]
